# Supplementary material for: Adaptive Bitrate Streaming Over Cellular Networks: Rate Adaptation and Data Savings Strategies
Source: arXiv:2104.01104 source file (2021-05-14)
Supplement: Supplementary file 1 [file appendix.tex]

% \newpage
%\begin{appendix}\label{sec:appendx}
%\section{Bitrate of Audio and Video Combinations}

%\end{appendix} 
